# Supplementary material for: Towards Enabling I/O Awareness in Task-based Programming Models
Source: arXiv:2111.01504 source file (2021-11-02)
Supplement: Supplementary file 1 [file appendix.tex]

\appendix

\section{Learning Phases of the Variant Discovery Pipeline I/O Tasks}
